# Supplementary material for: Ordered Topological Deep Learning: a Network Modeling Case Study
Source: arXiv:2503.16746 source file (2025-03-20)
Supplement: Supplementary file 1 [file applicability.tex]

TODO: introductory paragraph

\paragraph{Scheduling Policies.} In order to ensure that specific traffic flows meet performance guarantees such as low latency, high throughput, or prioritized delivery, RouteNet is compatible with different queue scheduling policies, enabling to allocate resources among flows based on their priorities. %Some implemented policies are First In, First Out (FIFO), Weighted Fair Queuing (WFQ), Deficit Round Robin (DRR), and Strict Priority (SP). 
Table~\ref{tab:scheduling_delay} shows the results of evaluating RouteNet in scenarios with mixed scheduling policies, demonstrating its ability to accurately predict delay under different traffic intensities and diverse scheduling configurations. %RouteNet-F significantly outperforms the QT benchmark, highlighting its robustness and adaptability in modeling networks with QoS and diverse scheduling configurations.

\begin{table}[!t]
\caption{Benchmark of QT and RouteNet in the presence of Scheduling Policies for low, medium, and high traffic intensity.}
\label{tab:scheduling_delay}
\centering
\resizebox{0.6\columnwidth}{!}{%
\begin{tabular}{ccccccccc}
\toprule
     & \multicolumn{3}{c}{Traffic Intensity} \\
     \cmidrule(lr){2-4}
     & Low & Medium  & High  \\
     \midrule
QT & 13.0\% & 17.3\% & 25.1\%  \\
RouteNet & 0.80\% & 2.60\% & 7.31\% \\
\bottomrule
\end{tabular}%
}
\end{table}

\begin{table}[!t]
\caption{Generalization results of RouteNet evaluated on increasing topology sizes. The model was trained with topologies of up to 10 nodes.}
\label{tab:generalization_comparison}
\centering
\resizebox{0.75\columnwidth}{!}{%
\begin{tabular}{ccccc}
\toprule
Topology Size & MAPE & MSE & MAE  \\
\midrule
50  & 0.76\% & 0.00004 & 0.001  \\
% 75  & 1.17\% & 0.00019 & 0.002 & 0.984 \\
100 & 1.89\% & 0.00016 & 0.003  \\
% 130 & 1.55\% & 0.00005 & 0.002 & 0.985 \\
% 170 & 2.43\% & 0.00008 & 0.002 & 0.978 \\
200 & 2.67\% & 0.00006 & 0.002  \\
% 240 & 2.58\% & 0.00007 & 0.002 & 0.979 \\
% 260 & 3.17\% & 0.00007 & 0.003 & 0.969 \\
% 280 & 3.16\% & 0.00003 & 0.002 & 0.979 \\
300 & 2.45\% & 0.00003 & 0.001  \\
\bottomrule
\end{tabular}%
}
\end{table}

\paragraph{Scalability.}
Scalability is a key challenge in data-driven network modeling. Unlike analytical methods like QT, which rely on assumptions, data-driven models require training datasets capturing diverse network conditions. However, production networks rarely experience extreme conditions such as severe congestion or link failures, making it challenging to generate such datasets in operational settings. 
Controlled testbeds provide an effective alternative, allowing for the creation of synthetic datasets that replicate a wide range of network behaviors. However, network testbeds are usually much smaller than real networks. 
%RouteNet, trained on such diverse datasets, has demonstrated its ability to generalize effectively, accurately predicting performance even in scenarios involving previously unseen routing configurations or topologies. This generalization capability is essential for adapting to the dynamic nature of real-world networks. 
To validate RouteNet’s ability to scale to larger networks, the model was trained on small topologies with up to 10 nodes and then evaluated on networks of increasing size, ranging from 50 to 300 nodes. Table~\ref{tab:generalization_comparison} summarizes the results, showing that RouteNet consistently achieves low error rates, even for networks 30x larger than those seen during training. 
%For example, the MAPE remains below 3.17\% for all topology sizes, with minimal differences from previous experiments. These results highlight RouteNet's robustness and adaptability, demonstrating its capacity to scale to significantly larger networks while maintaining high prediction accuracy.

\begin{table}[!t]
\caption{Windowed Performance Metrics per Dataset}
\label{tab:performance_metrics}
\centering
\resizebox{0.7\columnwidth}{!}{%
\begin{tabular}{lcccc}
\toprule
{Dataset} & {Model} & {MAPE} & {MAE}  \\
\midrule
\multirow{2}{*}{{Synthetic}} 
    & OMNeT++ & 53.68\% & 63.4857  \\ 
    & RN-G    & 2.60\% & 3.1283  \\ 
\midrule
\multirow{2}{*}{{Multi-Burst}} 
    & OMNeT++ & 56.12\% & 67.8069  \\ 
    & RN-G    & 2.28\% & 2.8090   \\ 
\midrule
\multirow{2}{*}{{RWPT}} 
    & OMNeT++ & 93.08\% & 126.0875  \\ 
    & RN-G    & 14.75\% & 47.2170   \\ 
\bottomrule
\end{tabular}%
}
\end{table}

\paragraph{Non-Stationary Traffic}
Real-world networks often experience non-stationary traffic, where traffic patterns evolve due to changes in user behavior, network conditions, or external factors. Traditional RouteNet models are limited to predicting aggregate performance metrics over the duration of a flow, making them less suited for capturing temporal variations in traffic. 
To address this limitation, the latest RouteNet version %a recent version of RouteNet, RouteNet-Gauss~\cite{güemespalau2025routenetgausshardwareenhancednetworkmodeling}, 
introduces a temporal component. By dividing network scenarios into fixed-size windows and processing each window independently, it captures temporal dependencies and provides a detailed view of how flow performance metrics evolve. This advancement enables RouteNet to handle dynamic and non-stationary traffic patterns, a critical requirement for real-world network management. 
Table~\ref{tab:performance_metrics} presents the performance of RouteNet compared to the OMNeT++ simulator across three datasets that reflect varying traffic dynamics: Synthetic traffic with high-frequency bursts, Multi-Burst traffic, and Real-World Packet Traces (RWPT). 
% [SUMMARIZE RESULTS IN A HEADLINE]
Overall, RouteNet proved to be more faithful while replicating the packet's behavior than the OMNeT++ simulator, both in synthetic and real traffic distributions, decreasing the MAPE by 84\% in the latter.
%While machine learning models like RouteNet-Gauss demonstrate strong performance across these datasets, OMNeT++ exhibits significantly higher error rates, particularly for more complex traffic patterns such as RWPT. This discrepancy highlights a common limitation of traditional network simulators like OMNeT++, which are designed to operate under idealized conditions with controlled and well-defined traffic assumptions. However, real-world network environments often deviate from these idealizations due to dynamic and non-stationary factors such as bursty traffic, unexpected congestion, and varying flow priorities. As a result, simulators like OMNeT++ struggle to maintain accuracy when faced with the variability and complexity of real-world conditions, underscoring the need for adaptive, data-driven approaches like RouteNet-Gauss.

% \paragraph{Deployment.} [MAYBE MENTION FEASIBILITY OF DEPLOYMENT? HIGHLIGHTING ALL PREVIOUS FEATURES]
